# Supplementary material for: Natural Language Induced Adversarial Images
Source: arXiv:2410.08620 source file (2024-10-11)
Supplement: Supplementary file 1 [file ZHU_SM_camera_2.0.pdf]

# Supplementary Materials: Natural Language Induced Adversarial Images

Xiaopei Zhu
Department of Computer Science & Technology, Tsinghua University
Beijing, China
zxpthu@gmail.com

Peiyang Xu*
Department of Computer Science & Technology, Tsinghua University
Beijing, China
xupy21@mails.tsinghua.edu.cn

Guanning Zeng
Department of Computer Science & Technology, Tsinghua University
Beijing, China
zgn21@mails.tsinghua.edu.cn

Yingpeng Dong
Department of Computer Science & Technology, Tsinghua University
Beijing, China
dongyinpeng@mail.tsinghua.edu.cn

Xiaolin Hu†‡
Department of Computer Science & Technology, Tsinghua University.
Beijing, China
xlhu@tsinghua.edu.cn

**ACM Reference Format:**
Xiaopei Zhu, Peiyang Xu, Guanning Zeng, Yingpeng Dong, and Xiaolin Hu. 2024. Supplementary Materials: Natural Language Induced Adversarial Images. In *Proceedings of the 32nd ACM International Conference on Multimedia (MM'24), October 28-November 1, 2024, Melbourne, Australia.* ACM, New York, NY, USA, 5 pages. https://doi.org/10.1145/3664647.3680902

## 1 PROMPT STRUCTURE AND WORD SPACE SETTINGS

The adversarial prompt structure and word space is customizable, which can be either manually designed or auto-generated by GPT-4 for initialization. In our experiments, we manually designed the adversarial prompt structures and word spaces for the animal and race classification attack tasks. Then we introduce the auto-generation method by using GPT-4. We chose the vehicle target as an example. The details are provided as follows.

### 1.1 Attack Animal Classifiers

**Prompt Structure:**

*"<number><color>[target animal] <appearance>is <gesture>on the <background>on a <weather>day, the [target animal] faces forward, the [target animal] occupies the main part in this scene, viewed <viewangle>."*

*"<word>"* represents a word that can be optimized. *"[target animal]"* is the ground truth target category $y$ (e.g. "cat") of the generated images, which is user-defined and fixed during the prompt optimization.

*Equal contribution with Xiaopei Zhu
†Corresponding Author
‡Institute for Artificial Intelligence, BNRist, THBI, IDG/McGovern Institute for Brain Research, Tsinghua University, Beijing, China.
Chinese Institute for Brain Research (CIBR), Beijing, China.

Permission to make digital or hard copies of part or all of this work for personal or classroom use is granted without fee provided that copies are not made or distributed for profit or commercial advantage and that copies bear this notice and the full citation on the first page. Copyrights for third-party components of this work must be honored. For all other uses, contact the owner/author(s).
*MM '24, October 28-November 1, 2024, Melbourne, VIC, Australia*
© 2024 Copyright held by the owner/author(s).
ACM ISBN 979-8-4007-0686-8/24/10
https://doi.org/10.1145/3664647.3680902

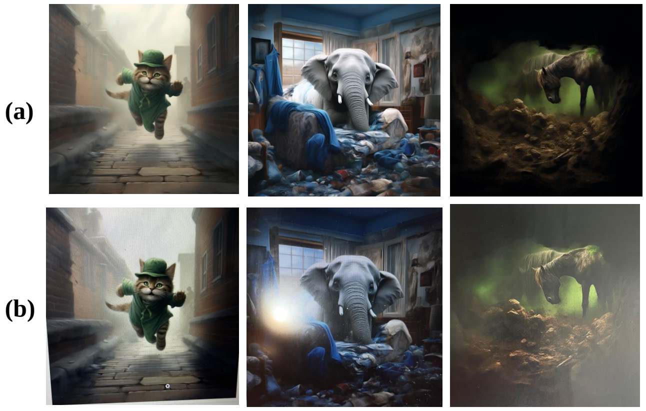


**Figure S1: Comparison of (a) digital and (b) physical adversarial images.**

**Word Space:** The specific settings for the word space in the animal classification attacks are introduced in Table S1.

### 1.2 Attack Race Classifiers

**Prompt Structure:**

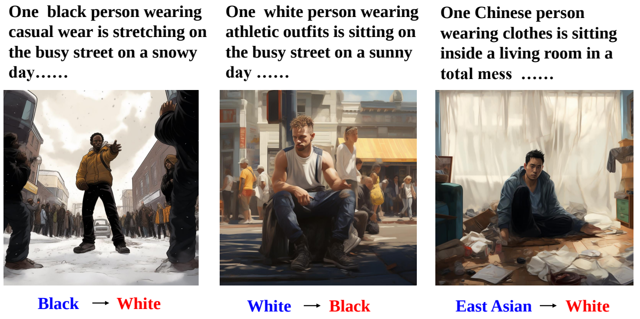


**Figure S2: Examples of human race classification attacks.**

**Table S1: Word space setting for the animal classifier attack**

| Attribute | Value | | |
|---|---|---|---|
| number | one | two | many |
| color | red | blue | green |
| | yellow | black | white |
| | purple | orange | brown |
| | many different colors | | |
| target animal | butterfly | cat | chicken |
| | cow | dog | elephant |
| | horse | sheep | spider |
| | squirrel | | |
| appearance | wearing a hat | wearing a pair of glasses | wearing clothes |
| | wearing a flower on the head | | |
| gesture | sitting | flying | taking a nap |
| | running | playing with a ball | chasing a butterfly |
| | digging a burrow | crawling | stretching |
| | barking | standing | |
| background | on the sky covered with clouds | on the green grass field with flowers | on Mars |
| | on the ground covered with snow and ice | on the busy street | in front of a brick wall |
| | inside a living room which is in a total mess | in the dense forest | in the rocky terrain |
| | under the deep sea | on the moon | |
| weather | sunny | rainy | cloudy |
| | snowy | windy | foggy |
| | stormy | humid | |
| view angle | from an eye-level perspective | | |
| style | blank | blurry, fuzzy, misty | realistic |

*“<number><expression>[target person] <appearance>is <gesture>on the <background>on a <weather>day, the [target person] >faces forward, the [target person] occupies the main part in this scene, viewed <view angle>, in a <style>."*

*“<word>”* represents a word that can be optimized. *“[target person]”* is the ground truth target category $y$ (e.g. “white person”) of the generated images, which is user-defined and fixed during the prompt optimization.

**Word Space:** The specific settings for the word space in the race classification attacks are introduced in the Table S2.

## 1.3 Auto-Generation Mehtod

The word space is a fundamental component of our attack pipeline. Since it needs to be adapted to different classification tasks, manually crafting a word space for each task requires a lot of effort. To address this issue, we use GPT-4 to auto-generate the word space. First, we can select a new target category, such as vehicle, road sign, etc. Next, the above hand-constructed word spaces are input into GPT-4 as examples, and GPT-4 is instructed to generate a similar word space for a new task.

The prompt used for auto-generating the word space by GPT-4 is shown as follows:

*Now I need you to help construct a word space for the given task task. Here are two examples of the constructed word space. First is for animal classification. The word space is: ‘number’: [‘one’,‘two’], ‘weather’: [‘sunny’, ‘rainy’, ‘cloudy’, ‘snowy’, ‘windy’, ‘foggy’, ‘stormy’, ‘humid’],‘background’:... And the second example is for human race classification. The word space is: ‘number’:[‘one’],‘weather’: ...*

*When constructing the word space, you can also think from the above perspectives. But pay attention that each task may have its unique feature, e.g. humans may wear various clothes but their skin colors are limited, and animals may have unique behaviours like barking or flying. When constructing word space, you must take these characteristics of different tasks into consideration and construct the most suitable word space. Do remember that your constructed word space should have the same attribute: number, weather, background, color, view angle, gesture, style, appearance, expression. If you find one attribute is not suitable for the task, you should keep the key and give a list [”] as its value. Now construct the word space for the task of task classification. Your answer must be in the form of a python dictionary like the example above. Do not include any words other than the dictionary!*

The auto-generated word space for the vehicle classification task is shown in Table S3. It shows that the generated word space has been adapted to the vehicle classification task. The pipeline of our mehtod is fully automated without manually designed component by using the auto-generation method.

## 1.4 Stability of the Attack

Since the generation of text-to-image models is a stochastic process, the same prompt may lead to different images in successive queries. To verify the stability of our attack method, we selected 10 optimized prompts, then inputted it into Midjourney 10 times,

**Table S2: Word space setting for the race classifier attack**

| Attribute | Value | | |
|---|---|---|---|
| number | one | two | many |
| expression | happy<br>worried | sad<br>depressed | angry<br>overwhelmed |
| target person | white person | black person | Chinese person |
| appearance | wearing a hat<br>wearing casual wear<br>with long hair<br>wearing a flower on the head<br>wearing earrings | wearing a pair of glasses<br>wearing traditional attires<br>with short hair<br>with tatoo on the face<br>wearing bracelets | wearing formal suits<br>wearing athletic outfits<br>with curly hair<br>wearing necklaces |
| gesture | sitting<br>running<br>digging a burrow<br>studying | smoking<br>playing with a ball<br>crawling<br>exercising | taking a nap<br>chasing a butterfly<br>stretching<br>working |
| background | on the sky covered with clouds<br>on the ground with snow and ice<br>inside a living room in a total mess<br>under the deep sea | on the green grass field with flowers<br>on the busy street<br>in the dense forest<br>on the moon | on Mars<br>in front of a brick wall<br>in the rocky terrain |
| weather | sunny<br>snowy<br>stormy | rainy<br>windy<br>humid | cloudy<br>foggy |
| view angle | from an eye-level perspective | | |
| style | blank | blurry, fuzzy, misty | realistic |

**Table S3: Word space setting for the vehicle classifier attack**

| Attribute | Value | | |
|---|---|---|---|
| number | one<br>multiple | two | three |
| color | red<br>yellow<br>silver<br>brown | blue<br>black<br>gray | green<br>white<br>orange |
| target vehicle | bicycle<br>bus<br>underground | motorbike<br>truck | car<br>train |
| appearance | with headlights on<br>with a sunroof | with doors open<br>with tinted windows | with a spoiler |
| background | on the highway<br>in a garage<br>near a body of water<br>on a bridge | in a parking lot<br>on a race track<br>in a desert | on a city street<br>in a rural area<br>in a forest |
| weather | sunny<br>snowy<br>stormy | rainy<br>windy<br>humid | cloudy<br>foggy |
| view angle | from the front | from the side | from the back |
| style | blank | blurry, fuzzy, misty | realistic |

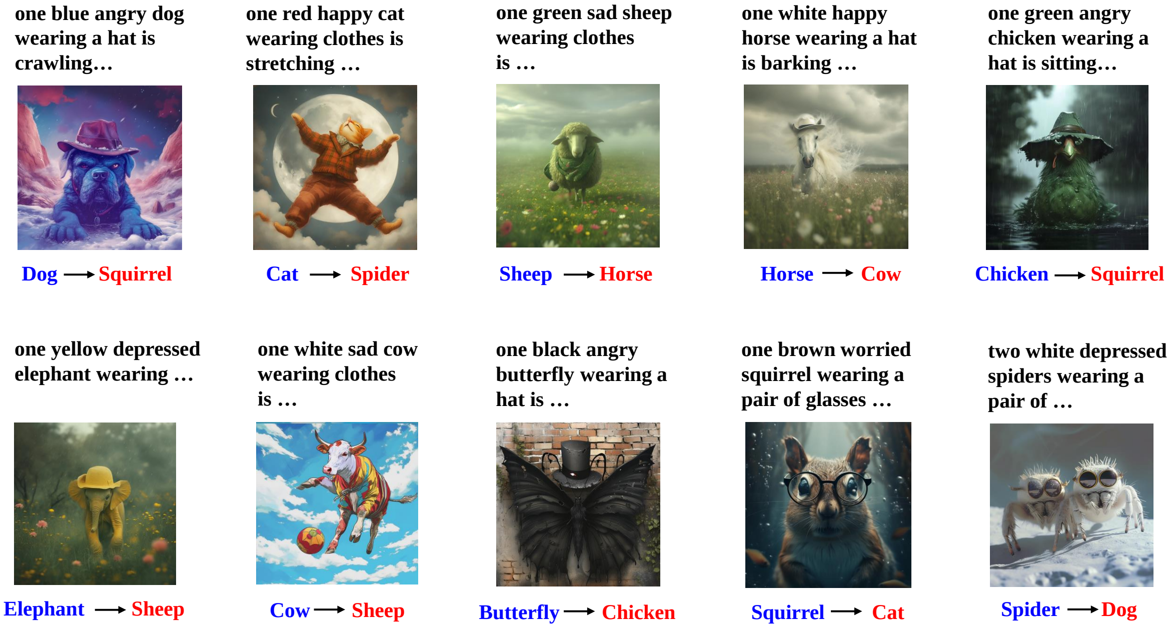


**Figure S3: Example images for attacking the animal classifier trained on ImageNet. The black texts are the prompts, the blue texts are the groundtruth categories, and the red texts are the misclassified categories.**

**Table S4: Attack Stability Verification.**

| Times | 1 | 2 | 3 | 4 | 5 | 6 | 7 | 8 | 9 | 10 | Average |
|---|---|---|---|---|---|---|---|---|---|---|---|
| ASR(%) | 87.5 | 77.5 | 85.0 | 92.5 | 87.5 | 75.0 | 90.0 | 82.5 | 82.5 | 85.0 | 84.5 ± 5.4 |

and tested the ASRs of the 40 generated adversarial images each time. The results are shown in Table S4. It indicates that the ASRs of our adversarial prompts were higher than 75% in 10 successive attacks. The average ASR was 84.5% ± 5.4%. This shows that our attack method has good stability. Moreover, This suggests that, to a certain extent, our method can find the key semantic information in the natural language space, and adversarial images with such semantic information have stable adversarial effects.

## 2 DETAILS FOR SEARCHING ADVERSARIAL IMAGES BY GOOGLE

We searched for some photos captured in the real world on Google according to the adversarial semantic information analyzed by our method. For example, we obtained 50 images returned by Google with 10 prompts like "A cat is stretching", "A horse in a foggy day", etc. For fair comparison, we also searched 50 images by Google using prompts with random word selection as control experiments. For each prompt, we select pictures with top-5 semantic relevance ranking in Google, and we checked whether they were real photos based on the source of the picture provided by Google. For example, if the picture came from a news report or a photography competition, we regarded it as a real photo. We only retained photos that came from these reliable sources.

### 2.1 Physical Attacks

We tested the attack effect of our method in the physical world. We selected 40 adversarial images obtained in Section 4.5 of main paper, which successfully misled the ResNet101 classifier. Using a Canon MF657 printer, we printed these images and then captured them with iPhone 12 Pro from a distance of 30 cm. Examples of the digital and physical images are shown in Figure S1. We inputted the captured photos into the ResNet101 classifier and calculated the ASR. The results indicated that our method achieved a 100% ASR both in the digital and physical worlds. The physical world adds more perturbations [3] to the images, e.g. the printer may cause color distribution variations [1], usually leading to lower physical ASRs for previous noise-based [2] or image editing-based [4] approaches compared to their digital ASRs. However, our method are based on language with explicit semantic information, and therefore may be more robust in the physical world.

## 3 DETAILS OF THE ATTACKS ON RACE CLASSIFIER

We evaluated the attack effect of our method on 3-race classification tasks (black, white, east asian). We chose Midjourney as the text-to-image generator for adversarial images. The settings for the adversarial prompt structure and word space are introduced in Section S1.2. Our adaptive GA method was used to generate

adversarial prompts and images. For each target race, we set the population size to 20. The mutation probability was set to 0.01, and the hyperparameter $\lambda$ in the fitness function was set to 0.5. The termination condition was that the number of iterations reached 15 generations. We obtained adversarial prompts and images by using the above method. The ASR of the adversarial images against the human race classifier Vit was 89%, and some examples are shown in Figure S2. It indicates that our method effectively attacked the race classifier Vit.

## 4 EXAMPLE IMAGES FOR ATTACKING THE CLASSIFIER TRAINED ON IMAGENET

Figure S3 shows a set of a examples of adversarial prompts and images for attacking the animal classifier ResNet101 trained on ImageNet.

## REFERENCES

[1] Kevin Eykholt, Ivan Evtimov, Earlence Fernandes, Bo Li, Amir Rahmati, Chaowei Xiao, Atul Prakash, Tadayoshi Kohno, and Dawn Song. 2018. Robust physical-world attacks on deep learning visual classification. In *Proceedings of the IEEE conference on computer vision and pattern recognition*. 1625–1634.

[2] Jiajun Lu, Hussein Sibai, Evan Fabry, and David Forsyth. 2017. No need to worry about adversarial examples in object detection in autonomous vehicles. *arXiv preprint arXiv:1707.03501* (2017).

[3] Simen Thys, Wiebe Van Ranst, and Toon Goedemé. 2019. Fooling automated surveillance cameras: adversarial patches to attack person detection. In *Proceedings of the IEEE/CVF conference on computer vision and pattern recognition workshops*. 0–0.

[4] Donghua Wang, Wen Yao, Tingsong Jiang, Guijian Tang, and Xiaoqian Chen. 2022. A survey on physical adversarial attack in computer vision. *arXiv preprint arXiv:2209.14262* (2022).
